# Supplementary material for: Online Double Oracle
Source: arXiv:2103.07780 source file (2023-02-15)
Supplement: Supplementary file 1 [file Appendix.pdf]

Supplementary Material for Online Double Oracle

Contents

A Online Single Oracle 2

A.1 Proof of Lemma 1 2

A.2 Proof of Theorem 5 2

A.3 Online Single Oracle with Slowly Adding New Strategy 3

B Online Double Oracle 4

B.1 Proof of Theorem 6 4

B.2 Proof of Lemma 7 5

B.3 Proof of Theorem 8 5

B.4 Prod Algorithm with Online Single Oracle 7

C Additional Results to Experiment Section 8

C.1 Convergence to NE in Asymmetric Games 8

C.2 Convergence to NE in Real-World Zero-Sum Games 9

## A. Online Single Oracle

### A.1. Proof of Lemma 1

**Lemma.** Suppose the matrix  $A_{n \times m}$  has a unique Nash equilibrium  $(\pi^*, c^*)$ , then the support of the Nash equilibrium of the row player will follow:

$$\max(|\text{supp}(\pi^*)|, |\text{supp}(c^*)|) \leq \min(n, m),$$

where  $|\cdot|$  denotes the cardinality of a set.

*Proof.* Since the size of  $\pi^*$  and  $c^*$  are  $n$  and  $m$  respectively, the size of the support of NE can not exceed the size of the game:

$$|\text{support}(\pi^*)| \leq n; |\text{support}(c^*)| \leq m.$$

In the case the game  $A$  has a unique Nash equilibrium, following Theorem 1 in (Bohnenblust et al., 1950), we have:

$$|\text{support}(\pi^*)| = |\text{support}(c^*)| \leq \min(n, m).$$

Thus, we have proved the lemma.  $\square$

### A.2. Proof of Theorem 5

**Theorem (Regret Bound of OSO).** Let  $l_1, l_2, \dots, l_T$  be a sequence of loss vectors played by an adversary. Then, OSO in Algorithm 2 is a no-regret algorithm with:

$$\frac{1}{T} \left( \sum_{t=1}^T \langle \pi_t, l_t \rangle - \min_{\pi \in \Pi} \sum_{t=1}^T \langle \pi, l_t \rangle \right) \leq \frac{\sqrt{k \log(k)}}{\sqrt{2T}},$$

where  $k = |\Pi_T|$  is the size of effective strategy set in the final time window.

*Proof.* W.l.o.g, we assume the player uses the MWU as the no-regret algorithm and starts with only one pure strategy in  $\Pi_0$  in Algorithm 2. Since in the final time window, the effective strategy set has  $k$  elements, there are exactly  $k$  time windows. Denote  $|T_1|, |T_2|, \dots, |T_k|$  be the lengths of time windows during each of which the subset of strategies the no-regret algorithm considers does not change. In the case of finite set of strategies,  $k$  will be finite and we have

$$\sum_{i=1}^k |T_i| = T. \quad (1)$$

In the time window with length  $|T_i|$ , following the regret bound of MWU in equation (5) we have:

$$\sum_{t=|\bar{T}_i|+1}^{|\bar{T}_{i+1}|} \langle \pi_t, l_t \rangle - \min_{\pi \in \Pi_{|\bar{T}_i|+1}} \sum_{t=|\bar{T}_i|+1}^{|\bar{T}_{i+1}|} \langle \pi, l_t \rangle \leq \sqrt{\frac{|T_i|}{2} \log(i)}, \quad \text{where } |\bar{T}_i| = \sum_{j=1}^{i-1} |T_j|. \quad (2)$$

In the time window  $T_i$ , we consider the full strategy set when we calculate the best response strategy in step 11 of Algorithm 2 and it stays in  $\Pi_{|\bar{T}_i|+1}$ . Therefore, the inequality (2) can be expressed as:

$$\sum_{t=|\bar{T}_i|+1}^{|\bar{T}_{i+1}|} \langle \pi_t, l_t \rangle - \min_{\pi \in \Pi} \sum_{t=|\bar{T}_i|+1}^{|\bar{T}_{i+1}|} \langle \pi, l_t \rangle \leq \sqrt{\frac{|T_i|}{2} \log(i)}. \quad (3)$$

Sum up the inequality (3) for  $i = 1, \dots, k$  we have:

$$\begin{aligned} \sum_{i=1}^k \sqrt{\frac{|T_i|}{2}} \log(i) &\geq \sum_{t=1}^T \langle \pi_t, l_t \rangle - \sum_{i=1}^k \min_{\pi \in \Pi} \sum_{t=|T_i|+1}^{|T_{i+1}|} \langle \pi, l_t \rangle \\ &\geq \sum_{t=1}^T \langle \pi_t, l_t \rangle - \min_{\pi \in \Pi} \sum_{i=1}^k \sum_{t=|T_i|+1}^{|T_{i+1}|} \langle \pi, l_t \rangle \end{aligned} \quad (4a)$$

$$\begin{aligned} &= \sum_{t=1}^T \langle \pi_t, l_t \rangle - \min_{\pi \in \Pi} \sum_{t=1}^T \langle \pi, l_t \rangle \\ &\Rightarrow \sqrt{\frac{Tk \log(k)}{2}} \geq \sum_{t=1}^T \langle \pi_t, l_t \rangle - \min_{\pi \in \Pi} \sum_{t=1}^T \langle \pi, l_t \rangle. \end{aligned} \quad (4b)$$

Inequality (4a) is due to  $\sum \min \leq \min \sum$ . Inequality (4b) comes from Cauchy-Schwarz inequality and Stirling' approximation. Thus, we have the derived regret.  $\square$

### A.3. Online Single Oracle with Slowly Adding New Strategy

---

#### Algorithm 1 Online Single Oracle with Slowly Adding New Strategy

---

```

1: Input: A set  $\Pi$  pure strategy set of player
2:  $\Pi_0 := \Pi_1$ : initial set of effective strategies
3: for  $t = 1$  to  $\infty$  do
4:   if  $\Pi_t = \Pi_{t-1}$  then
5:     Following the MWU update in Equation (4)
6:   else if  $\Pi_t \neq \Pi_{t-1}$  then
7:     Start a new time window  $T_{i+1}$ 
8:     Reset the MWU update in Equation (4) with a new initial strategy  $\pi_t$ 
9:   end if
10:  Observe  $l_t$  and update the average loss in the current time window  $T_i$ 
11:     $\bar{l} = \frac{1}{|T_i|} \sum_{\pi_t \in T_i} l_t$ 
12:  Calculate the best response:
13:     $a = \arg \min_{\pi \in \Pi} \langle \pi, \bar{l} \rangle$ ,
14:  if  $\min_{\pi \in \Pi_{|T_i|+1}} \langle \pi, \sum_{j=|T_i|}^t l_j \rangle - \min_{\pi \in \Pi} \langle \pi, \sum_{j=|T_i|}^t l_j \rangle \geq \alpha_{t-|T_i|}^i$  then
15:    Update the strategy set:  $\Pi_{t+1} = \Pi_t \cup a$ 
16:  else
17:     $\Pi_{t+1} = \Pi_t$ 
18:  end if
19:  Output the strategy  $\pi_t$  at round  $t$  for the player
20: end for
    
```

---

**Theorem** (Regret Bound of OSO with Slowly Adding New Strategy). *Let  $l_1, l_2, \dots, l_T$  be a sequence of loss vectors played by an adversary. Then, OSO in Algorithm 1 is a no-regret algorithm with:*

$$\frac{1}{T} \left( \sum_{t=1}^T \langle \pi_t, l_t \rangle - \min_{\pi \in \Pi} \sum_{t=1}^T \langle \pi, l_t \rangle \right) \leq \frac{\sqrt{k \log(k)}}{\sqrt{2T}} + \frac{\sum_{i=1}^k \alpha_{|T_i|}^i}{T},$$

where  $k = |\Pi_T|$  is the size of effective strategy set in the final time window.

*Proof.* W.l.o.g, we assume the player uses the MWU as the no-regret algorithm and starts with only one pure strategy in  $\Pi_0$  in Algorithm 2. Since in the final time window, the effective strategy set has  $k$  elements, there are exactly  $k$  time

windows. Denote  $|T_1|, |T_2|, \dots, |T_k|$  be the lengths of time windows during each of which the subset of strategies the no-regret algorithm considers does not change. In the case of finite set of strategies,  $k$  will be finite and we have

$$\sum_{i=1}^k |T_i| = T.$$

In the time window with length  $|T_i|$ , following the regret bound of MWU in equation (5) we have:

$$\sum_{t=|T_i|+1}^{|\bar{T}_{i+1}|} \langle \pi_t, \mathbf{l}_t \rangle - \min_{\pi \in \Pi_{|\bar{T}_i|+1}} \sum_{t=|T_i|+1}^{|\bar{T}_{i+1}|} \langle \pi, \mathbf{l}_t \rangle \leq \sqrt{\frac{|T_i|}{2} \log(i)}, \quad \text{where } |\bar{T}_i| = \sum_{j=1}^{i-1} |T_j|. \quad (5)$$

Since in the time window  $T_i$ , the size of the effective strategy set does not change, thus we have:

$$\min_{\pi \in \Pi_{|\bar{T}_i|+1}} \sum_{t=|T_i|+1}^{|\bar{T}_{i+1}|} \langle \pi, \mathbf{l}_t \rangle - \min_{\pi \in \Pi} \sum_{t=|T_i|+1}^{|\bar{T}_{i+1}|} \langle \pi, \mathbf{l}_t \rangle \leq \alpha_{|T_i|}^i \quad (6)$$

From Inequalities (5) and (6) we have:

$$\sum_{t=|T_i|+1}^{|\bar{T}_{i+1}|} \langle \pi_t, \mathbf{l}_t \rangle - \min_{\pi \in \Pi} \sum_{t=|T_i|+1}^{|\bar{T}_{i+1}|} \langle \pi, \mathbf{l}_t \rangle \leq \sqrt{\frac{|T_i|}{2} \log(i)} + \alpha_{|T_i|}^i \quad (7)$$

Sum up the inequality (7) for  $i = 1, \dots, k$  we have:

$$\begin{aligned} \sum_{i=1}^k \left( \sqrt{\frac{|T_i|}{2} \log(i)} + \alpha_{|T_i|}^i \right) &\geq \sum_{t=1}^T \langle \pi_t, \mathbf{l}_t \rangle - \sum_{i=1}^k \min_{\pi \in \Pi} \sum_{t=|T_i|+1}^{|\bar{T}_{i+1}|} \langle \pi, \mathbf{l}_t \rangle \\ &\geq \sum_{t=1}^T \langle \pi_t, \mathbf{l}_t \rangle - \min_{\pi \in \Pi} \sum_{i=1}^k \sum_{t=|T_i|+1}^{|\bar{T}_{i+1}|} \langle \pi, \mathbf{l}_t \rangle = \sum_{t=1}^T \langle \pi_t, \mathbf{l}_t \rangle - \min_{\pi \in \Pi} \sum_{i=1}^T \langle \pi, \mathbf{l}_t \rangle \end{aligned} \quad (8a)$$

$$\Rightarrow \sqrt{\frac{Tk \log(k)}{2}} + \sum_{i=1}^k \alpha_{|T_i|}^i \geq \sum_{t=1}^T \langle \pi_t, \mathbf{l}_t \rangle - \min_{\pi \in \Pi} \sum_{i=1}^T \langle \pi, \mathbf{l}_t \rangle. \quad (8b)$$

Inequality (8a) is due to  $\sum \min \leq \min \sum$ . Inequality (8b) comes from Cauchy-Schwarz inequality and Stirling' approximation. Thus, we have the derived regret bound.  $\square$

## B. Online Double Oracle

### B.1. Proof of Theorem 6

**Theorem.** Suppose both players use ODO algorithm. Let  $k_1, k_2$  denote the size of effective strategy set for row and column player, respectively. Then, the average strategies of both players converge to the Nash equilibrium with the rate:

$$\epsilon_T = \sqrt{\frac{k_1 \log(k_1)}{2T}} + \sqrt{\frac{k_2 \log(k_2)}{2T}}.$$

*Proof.* Using the regret bound of OSO algorithm in Theorem 5 we have:

$$\begin{aligned} \sum_{t=1}^T \pi_t^\top \mathbf{A} \mathbf{c}_t - \min_{\pi \in \Pi} \sum_{t=1}^T \pi^\top \mathbf{A} \mathbf{c}_t &\leq \sqrt{\frac{Tk_1 \log(k_1)}{2}}, \\ \max_{\mathbf{c} \in C} \sum_{t=1}^T \pi_t^\top \mathbf{A} \mathbf{c} - \sum_{t=1}^T \pi_t^\top \mathbf{A} \mathbf{c}_t &\leq \sqrt{\frac{Tk_2 \log(k_2)}{2}}. \end{aligned}$$

From the above inequalities we can derive that

$$\begin{aligned}\bar{\pi}^\top \mathbf{A}\bar{\mathbf{c}} &\geq \min_{\pi \in \Pi} \pi^\top \mathbf{A}\bar{\mathbf{c}} \geq \frac{1}{T} \sum_{t=1}^T \pi_t^\top \mathbf{A}\mathbf{c}_t - \sqrt{\frac{k_1 \log(k_1)}{2T}} \\ &\geq \max_{\mathbf{c} \in C} \sum_{t=1}^T \bar{\pi}^\top \mathbf{A}\mathbf{c} - \sqrt{\frac{k_2 \log(k_2)}{2T}} - \sqrt{\frac{k_1 \log(k_1)}{2T}}.\end{aligned}$$

Similarly, we have

$$\begin{aligned}\bar{\pi}^\top \mathbf{A}\bar{\mathbf{c}} &\leq \max_{\mathbf{c} \in C} \bar{\pi}^\top \mathbf{A}\mathbf{c} \leq \frac{1}{T} \sum_{t=1}^T \pi_t^\top \mathbf{A}\mathbf{c}_t + \sqrt{\frac{k_2 \log(k_2)}{2T}} \\ &\leq \min_{\pi \in \Pi} \pi^\top \mathbf{A}\bar{\mathbf{c}} + \sqrt{\frac{k_1 \log(k_1)}{2T}} + \sqrt{\frac{k_2 \log(k_2)}{2T}}.\end{aligned}$$

Thus, with  $\epsilon_T = \sqrt{\frac{T k_1 \log(k_1)}{2}} + \sqrt{\frac{T k_2 \log(k_2)}{2}}$  we have

$$\max_{\mathbf{c} \in C} \sum_{t=1}^T \bar{\pi}^\top \mathbf{A}\mathbf{c} - \epsilon_T \leq \bar{\pi}^\top \mathbf{A}\bar{\mathbf{c}} \leq \min_{\pi \in \Pi} \pi^\top \mathbf{A}\bar{\mathbf{c}} + \epsilon_T.$$

By definition,  $(\bar{\pi}, \bar{\mathbf{c}})$  is  $\epsilon_T$ -Nash equilibrium. □

## B.2. Proof of Lemma 7

**Lemma.** *The Double Oracle algorithm can still converge to  $\epsilon$ -Nash equilibrium if the players can only access to a  $\epsilon$ -best response in each round.*

*Proof.* We first prove in the case of oracle algorithm. The double oracle proof will be similar. Since the number of strategies is finite, by the same argument in the the case of exact best response, the process will converge. Suppose that at time step  $t$ , the process stops. Since we use  $\epsilon$ -best response, we have the following relationship:

$$\pi_t^\top \mathbf{A}_t \mathbf{l}_t - \min_{\pi \in \Pi} \pi^\top \mathbf{A}_t \mathbf{l}_t \leq \epsilon$$

If we set the weight of pure strategies does not appear in  $\pi_t$  to be zero to make a  $\pi'_t$ , then it is obvious that

$$\pi_t^\top \mathbf{A}_t = \pi'_t{}^\top \mathbf{A}$$

Thus, we have the following relationship:

$$\pi'_t{}^\top \mathbf{A} \mathbf{l}_t - \min_{\pi \in \Pi} \pi^\top \mathbf{A} \mathbf{l}_t \leq \epsilon \tag{9}$$

Further, since  $\mathbf{l}_t$  is Nash equilibrium of  $\mathbf{A}_t$ , we also have

$$\max_{l \in \Delta_l} \pi'_t{}^\top \mathbf{A} l - \pi'_t{}^\top \mathbf{A} \mathbf{l}_t = \max_{l \in \Delta_l} \pi_t^\top \mathbf{A}_t l - \pi_t^\top \mathbf{A}_t \mathbf{l}_t = 0 \tag{10}$$

From inequalities (9) and (10), by definition we conclude that  $(\pi'_t, \mathbf{l}_t)$  is  $\epsilon$ -Nash equilibrium of the game  $\mathbf{A}$ . □

## B.3. Proof of Theorem 8

**Theorem.** *Suppose the agent only accesses to  $\epsilon$ -best response in each iteration when following OSO algorithm 2. Then, if the adversary follows a no-regret algorithm then the average strategy of the agent will converge to  $\epsilon$ -Nash equilibrium:*

$$\max_{\mathbf{c} \in C} \bar{\pi}^\top \mathbf{A}\mathbf{c} - \epsilon \leq \bar{\pi}^\top \mathbf{A}\bar{\mathbf{c}} \leq \min_{\pi \in \Pi} \pi^\top \mathbf{A}\bar{\mathbf{c}} + \epsilon.$$

Furthermore, the algorithm is  $\epsilon$ -regret:

$$\lim_{T \rightarrow \infty} \frac{\max_{\pi \in \Delta_\Pi} R_T(\pi)}{T} \leq \epsilon.$$

*Proof.* Suppose that the player uses the Multiplicative Weights Update in Algorithm 2 with  $\epsilon$ -best response. Denote  $|T_1|, |T_2|, \dots, |T_k|$  be the lengths of time windows during each of which the subset of strategies the no-regret algorithm considers does not change. Furthermore,

$$\sum_{i=1}^k |T_i| = T.$$

In a time window  $T_i$ , the regret with respect to the best fixed strategy in the effective strategy set is:

$$\sum_{t=|\bar{T}_i|+1}^{|\bar{T}_{i+1}|} \langle \pi_t, l_t \rangle - \min_{\pi \in \Pi_{|\bar{T}_i|+1}} \sum_{t=|\bar{T}_i|+1}^{|\bar{T}_{i+1}|} \langle \pi, l_t \rangle \leq \sqrt{\frac{|T_i|}{2} \log(i)}, \quad (11)$$

where  $|\bar{T}_i| = \sum_{j=1}^{i-1} |T_j|$ . Since in the time window  $T_i$ , the  $\epsilon$ -best response strategy stays in  $\Pi_{\bar{T}_i+1}$  and therefore we have:

$$\min_{\pi \in \Pi_{|\bar{T}_i|+1}} \sum_{t=|\bar{T}_i|+1}^{|\bar{T}_{i+1}|} \langle \pi, l_t \rangle - \min_{\pi \in \Pi} \sum_{t=|\bar{T}_i|+1}^{|\bar{T}_{i+1}|} \langle \pi, l_t \rangle \leq \epsilon |T_i|$$

Then, from the inequality (11) we have:

$$\sum_{t=|\bar{T}_i|+1}^{|\bar{T}_{i+1}|} \langle \pi_t, l_t \rangle - \min_{\pi \in \Pi} \sum_{t=|\bar{T}_i|+1}^{|\bar{T}_{i+1}|} \langle \pi, l_t \rangle \leq \sqrt{\frac{|T_i|}{2} \log(i)} + \epsilon |T_i|, \quad (12)$$

Sum up the inequality (12) for  $i = 1, \dots, k$  we have:

$$\begin{aligned} \sum_{t=1}^T \langle \pi_t, l_t \rangle - \sum_{i=1}^k \min_{\pi \in \Pi} \sum_{t=|\bar{T}_i|+1}^{|\bar{T}_{i+1}|} \langle \pi, l_t \rangle &\leq \sum_{i=1}^k \sqrt{\frac{|T_i|}{2} \log(i)} + \epsilon T, \\ \Rightarrow \sum_{t=1}^T \langle \pi_t, l_t \rangle - \min_{\pi \in \Pi} \sum_{i=1}^k \sum_{t=|\bar{T}_i|+1}^{|\bar{T}_{i+1}|} \langle \pi, l_t \rangle &\leq \epsilon T + \sum_{i=1}^k \sqrt{\frac{|T_i|}{2} \log(i)} \end{aligned} \quad (13a)$$

$$\begin{aligned} \Rightarrow \sum_{t=1}^T \langle \pi_t, l_t \rangle - \min_{\pi \in \Pi} \sum_{t=1}^T \langle \pi, l_t \rangle &\leq \epsilon T + \sum_{i=1}^k \sqrt{\frac{|T_i|}{2} \log(i)} \\ \Rightarrow \sum_{t=1}^T \langle \pi_t, l_t \rangle - \min_{\pi \in \Pi} \sum_{t=1}^T \langle \pi, l_t \rangle &\leq \epsilon T + \sqrt{\frac{T}{2}} \sqrt{k \log(k)}. \end{aligned} \quad (13b)$$

Inequality (13a) is due to  $\sum \min \leq \min \sum$ . Inequality (13b) comes from Cauchy-Schwarz inequality and Stirling' approximation. Using inequality (13b), we have:

$$\min_{\pi \in \Pi} \langle \pi, \bar{l} \rangle \geq \frac{1}{T} \sum_{t=1}^T \langle \pi_t, l_t \rangle - \sqrt{\frac{k \log(k)}{2T}} - \epsilon. \quad (14)$$

That is, the OSO algorithm is  $\epsilon$ -regret in the case of  $\epsilon$ -best response.

Since the adversary follows a no-regret algorithm, we have:

$$\begin{aligned} \max_{l \in \Delta_L} \sum_{t=1}^T \langle \pi_t, l \rangle - \sum_{t=1}^T \langle \pi_t, l_t \rangle &\leq \sqrt{\frac{T}{2}} \sqrt{L \log(L)} \\ \Rightarrow \max_{l \in \Delta_L} \langle \bar{\pi}, l \rangle &\leq \frac{1}{T} \sum_{t=1}^T \langle \pi_t, l_t \rangle + \sqrt{\frac{L \log(L)}{2T}} \end{aligned} \quad (15)$$

Using the inequalities in (14) and (15) we have:

$$\begin{aligned}\langle \bar{\pi}, \bar{l} \rangle &\geq \min_{\pi \in \Pi} \langle \pi, \bar{l} \rangle \geq \frac{1}{T} \sum_{t=1}^T \langle \pi_t, l_t \rangle - \sqrt{\frac{k \log(k)}{2T}} - \epsilon \\ &\geq \max_{l \in \Delta_L} \langle \bar{\pi}, l \rangle - \sqrt{\frac{L \log(L)}{2T}} - \sqrt{\frac{k \log(k)}{2T}} - \epsilon\end{aligned}$$

Similarly, we also have:

$$\begin{aligned}\langle \bar{\pi}, \bar{l} \rangle &\leq \max_{l \in \Delta_L} \langle \bar{\pi}, l \rangle \leq \frac{1}{T} \sum_{t=1}^T \langle \pi_t, l_t \rangle + \sqrt{\frac{L \log(L)}{2T}} \\ &\leq \min_{\pi \in \Pi} \langle \pi, \bar{l} \rangle + \epsilon + \sqrt{\frac{k \log(k)}{2T}} + \sqrt{\frac{L \log(L)}{2T}}\end{aligned}$$

Take the limit  $T \rightarrow \infty$ , we then have:

$$\max_{l \in \Delta_L} \langle \bar{\pi}, l \rangle - \epsilon \leq \langle \bar{\pi}, \bar{l} \rangle \leq \min_{\pi \in \Pi} \langle \pi, \bar{l} \rangle + \epsilon$$

Thus  $(\bar{\pi}, \bar{l})$  is the  $\epsilon$ -Nash equilibrium of the game.  $\square$

#### B.4. Prod Algorithm with Online Single Oracle

Denote the OSO Algorithm 2 by  $A$  and the existing algorithm with regret bound  $R_B(T)$  by  $B$ . Then we have the following Prod Algorithm (?):

---

##### Algorithm 2 OSO-Prod algorithm

---

**Input:** learning rate  $\eta \in (0, 1/2]$ , initial weights  $w_{1,B}, w_{1,A}$ , num. of rounds  $T$ ;  
**for**  $t = 1, 2, \dots, T$  **do**  
    Let  $s_t = \frac{w_{t,B}}{w_{t,B} + w_{1,A}}$   
    Observe  $a_t$  and  $b_t$  and calculate  $x_t = s_t b_t + (1 - s_t) a_t$   
    Observe  $f_t$  and suffer loss  $l_t(x_t)$   
    Feed  $l_t$  to  $A$  and  $B$   
    Compute  $\delta_t = l_t(a_t) - l_t(b_t)$  and set  $w_{t+1,B} = w_{t,B}(1 + \eta \delta_t)$   
**end for**

---

**Theorem** (Theorem 9). *Following the OSO-Prod algorithm with the learning rate  $\eta = \frac{1}{2} \sqrt{(\log(T)/T)}$  and  $w_{1,A} = 1 - w_{1,B} = 1 - \eta$  guarantees the regret bound  $R_T(\text{OSO-Prod})$  of*

$$\min(R_T(B) + 2\sqrt{T \log(T)}, \frac{T\sqrt{k \log(k)}}{2} + 2\log(2)).$$

The proof of Theorem 9 comes directly from Corollary 1 in ?. We provide the Corollary here for the completeness of the paper:

**Corollary 1** (Corollary 1 in (?)). *Let  $C \geq 1$  be an upper bound on the total benchmark loss  $L_T(A)$ . Then setting  $\eta = \frac{1}{2} \sqrt{\frac{\log(C)}{C}}$  and  $w_{1,A} = 1 - w_{1,B} = 1 - \eta$  simultaneously guarantees*

$$R_T((A, B) - \text{Prod}) \leq R_T(B) + 2\sqrt{C \log(C)}$$

and

$$R_T((A, B) - \text{Prod}) \leq R_T(A) + 2\log(2).$$

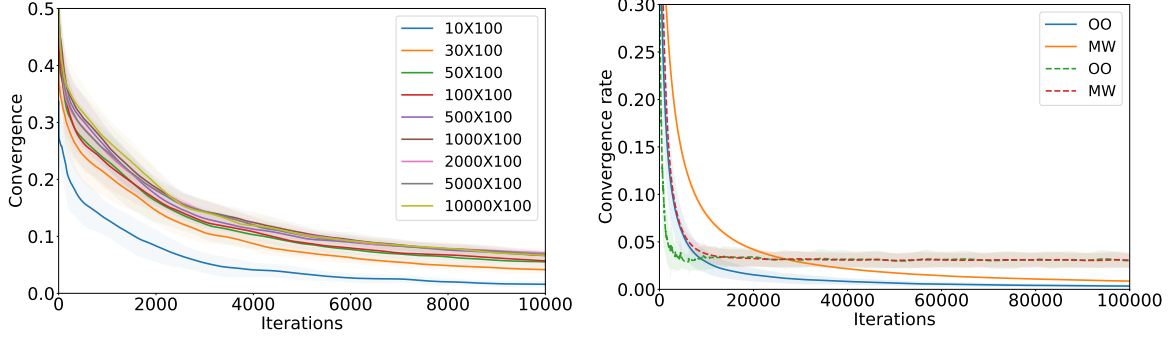

(a) Convergence to NE of OSO with different matrices' sizes (b) OSO algorithm vs MWU in an asymmetric game.

Figure 1. Results on Asymmetric Games.

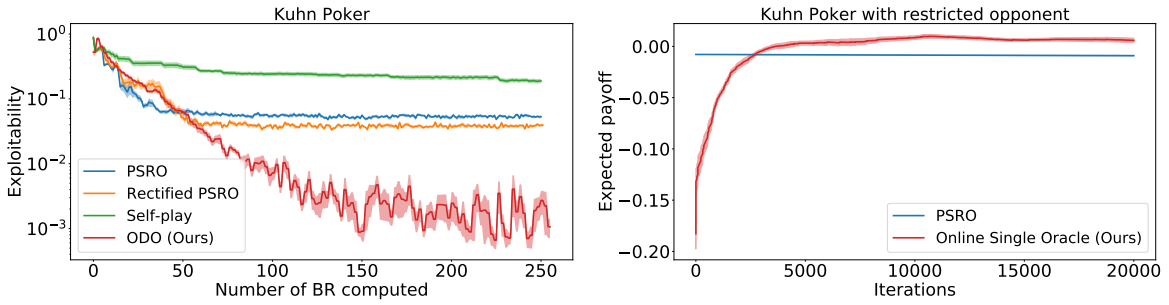

(a) Performance comparison in exploitability (b) Performance comparison in average payoff

Figure 2. Results on Kuhn Poker ( $2^{12}$  pure strategies).

## C. Additional Results to Experiment Section

We provide further experiments to demonstrate the performance of the Online Single Oracle and Online Double Oracle algorithms.

### C.1. Convergence to NE in Asymmetric Games

**Convergence to NE and Average Payoff in Asymmetric Games** First, we conduct simple proof concept experiments to demonstrate that the Online Single Oracle Algorithm (row player) can indeed converge to Nash equilibria empirically when playing against a no-regret algorithm (column player). Figure 1a measures the  $\epsilon$ -Nash distance between the time average policy and the Nash equilibrium when the row player follows the Online Single Oracle algorithm in different sizes of games. We randomly generate a matrix with different numbers of rows. Each entry of all those matrices is randomly sampled from a uniform distribution  $U(0, 1)$ . We repeat the experiments with 20 different random seeds for each size of matrices and plot the mean values as the solid lines with  $\pm$ std in the shaded area. As we can see, the time average policies learned by Online Single Oracle algorithm converge to Nash equilibria in all sizes of games. In this experiment, we fix the number of pure strategies of the column player (i.e., 100 pure strategies), and observe that the Online Single Oracle algorithm (row player) has roughly similar convergence rates regardless of its total number of pure strategies. This can be explained as since the number of pure strategies of the column player is fixed, the size of row player's effective strategy set is stable regardless the size of the full strategy set. Therefore, the Online Single Oracle Algorithm's convergence performance is less affected by its pure strategy set size.

We investigate into this problem and run another set of experiments in an extreme setting as follows (i.e., where  $k \log(k) < \log(n)$ ).

We consider a matrix of size  $10000 \times 3$  where we set the column player to always play by following the MWU algorithm. Figure 1b shows the convergence performance and the expected loss of the row player when it follows the Online Single Oracle and MWU algorithms. We can see that when the actual support of Nash policy is small, our algorithm will incur less loss and converge faster than normal no-regret algorithm.

Table 2. Nash Support of Games

| Game                      | Total Strategies | Size of Nash support |
|---------------------------|------------------|----------------------|
| 3-Move Parity Game 2      | 160              | 1                    |
| 5,4-Blotto                | 56               | 6                    |
| AlphaStar                 | 888              | 3                    |
| Connect Four              | 1470             | 23                   |
| Disc Game                 | 1000             | 27                   |
| Elo game + noise=0.1      | 1000             | 6                    |
| Elo game                  | 1000             | 1                    |
| Go (boardsize=3,komi=6.5) | 1933             | 13                   |
| Misere (game=tic tac toe) | 926              | 1                    |
| Normal Bernoulli game     | 1000             | 5                    |
| Quoridor (boardsize=3)    | 1404             | 1                    |
| Random game of skill      | 1000             | 5                    |
| Tic Tac Toe               | 880              | 1                    |
| Transitive game           | 1000             | 1                    |
| Triangular game           | 1000             | 1                    |

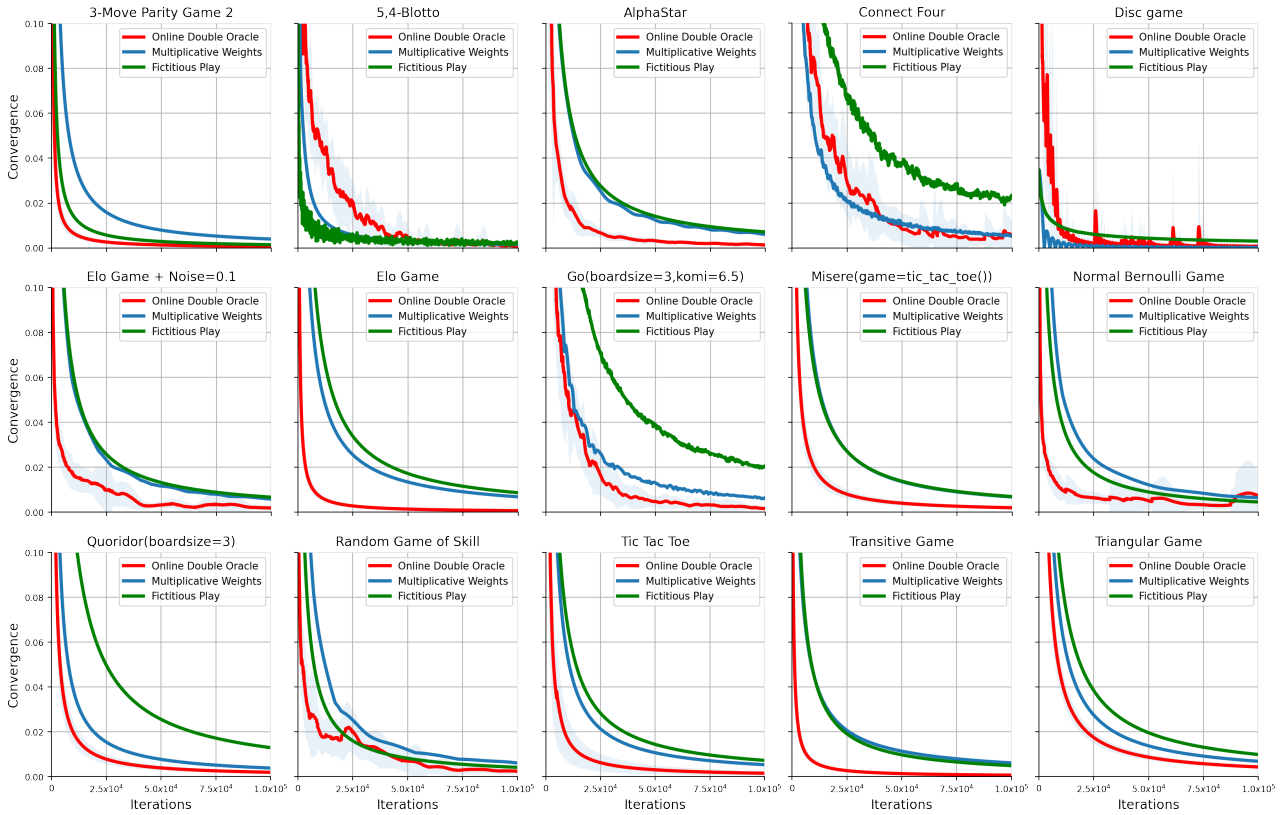

Figure 3. Online Double Oracle vs MWU and FP in symmetric games

## C.2. Convergence to NE in Real-World Zero-Sum Games

**Performance on Real-World Zero-Sum Games** We report the full results on the 15 popular real-world games and the support sizes of the NEs in these games in Figure 3 and Table 2.

**Large-Scale Games** We provide the experiment result for Kuhn Poker with  $2^{12}$  pure strategies. We can see a similar result to the Leduc poker experiment in Figure 2a, where the ODO shows a significant improvement in exploitability compared

to all the baselines. In average expected payoff test against the restricted opponent, the OSO also outperforms the PSRO in Kuhn Poker experiment (i.e., see Figure 2b). Since the size of Kuhn Poker is much smaller than Leduc Poker (i.e.,  $2^{12}$  against  $3^{936}$ ), a restricted opponent with 20 pure strategies is a much stronger player in Kuhn Poker than in Leduc Poker. Thus, as we can see in Figure 2b), it takes OSO longer to exploit the restricted opponent in Kuhn Poker compared to Leduc Poker.

## References

- Bohnenblust, H., Karlin, S., and Shapley, L. Solutions of discrete, two-person games. *Contributions to the Theory of Games*, 1:51–72, 1950.
- Sani, A., Neu, G., and Lazaric, A. Exploiting easy data in online optimization. In *Advances in Neural Information Processing Systems*, pp. 810–818, 2014.
